# Supplementary material for: Non-Markovian Models of Blocking in Concurrent and Countercurrent Flows
Source: arXiv:1303.4918 source file (2013-03-20)
Supplement: Supplementary file 1 [file supmat_v2.pdf]

# Supplementary Material: Non-Markovian Models of Blocking in Concurrent and Countercurrent Flows

A. Gabrielli, J. Talbot and P. Viot

March 19, 2013

## 1 Concurrent flow model

### 1.1 Rate equation approach

The most straightforward way to obtain the survival probability from Eqs. (2) is to solve them successively. However, because it will prove to be the most efficient method for the solution of the counterflow model, we show how the solution may be obtained using the generating function defined as

$$G(z,t) = \sum_{n=0}^{\infty} z^n q_s(n,t)\,.$$

Once this function is known, the survival probability is given simply by $p_s(t) = \sum_{n\geq 0} q_s(n,t) = G(1,t)$. By substituting the differential equations for $q_s(n,t)$, we can write

$$\frac{\partial G(z,t)}{\partial t} = z\lambda e^{-\lambda\tau} G(z,t-\tau) - \lambda G(z,t) + \lambda(z-1)e^{-\lambda t}\,.$$

Now taking the Laplace transform $\tilde{G}(z,u) = \int_0^\infty dt e^{-ut} G(z,t)$, we obtain

$$\tilde{G}(z,u) = \frac{1}{\lambda+u}\left[1 + \frac{\lambda z}{\lambda + u - \lambda z \exp(-(\lambda+u)\tau))}\right]\,.$$

While this cannot be directly inverted, by expanding the denominator we obtain:

$$\tilde{G}(z,u) = \frac{1}{\lambda+u} + \sum_{n=1}^{\infty} \frac{(\lambda z)^n}{(u+\lambda)^{n+1}} e^{-(n-1)\tau(\lambda+u)}\,.$$

Each term can now be inverted and one can verify that $G(1,t)$ gives Eq. (3). Note also that mean survival time can be obtained directly from the generating function

$$\langle t\rangle = \int_0^\infty t f(t) dt = \int_0^\infty p_s(t) dt = \tilde{G}(1,0) = \frac{2e^{\lambda\tau}-1}{\lambda(e^{\lambda\tau}-1)}\,.$$

### 1.2 Long time behavior

The long-time behavior of Eq. (3) can be obtained by considering the sum

$$I = \sum_{n=0}^{N} \frac{(\mu(N-n))^{n+1}}{(n+1)!}$$

where $\mu = \lambda\tau$. When $N$ is large, the sum can be approximated as

$$I \simeq \int_0^N dn \frac{(\mu(N-n))^{n+1}}{(n+1)!} \tag{S1}$$

By using the change of variable $\alpha = n/N$ and Stirling's Formula $m! \simeq \sqrt{2\pi m} m^m e^{-m}$, this can be expressed as

$$\begin{aligned} I &\simeq \frac{N^2\mu}{\sqrt{2\pi}} \int_0^1 d\alpha \frac{(1-\alpha)(\mu(N(1-\alpha))^{\alpha N}}{(\alpha N+1)\sqrt{\alpha}(\alpha N)^{\alpha N} e^{-\alpha N}} \\ &\simeq \frac{N^{3/2}\mu}{\sqrt{2\pi}} \int_0^1 d\alpha \frac{(1-\alpha)}{(\alpha N+1)\sqrt{\alpha}} \exp\left(-N\alpha \left[\ln\left(\frac{\alpha}{1-\alpha}\right) - 1 - \mu\right]\right) . \end{aligned}$$

For large $N$, the integral can be evaluated by the Laplace (saddle point) method. The extremum of the exponent in the preceding equation occurs at

$$\alpha^* = \frac{L_W(\mu)}{1 + L_W(\mu)} ,$$

where $L_W(x)$ is the Lambert function. Expanding the exponential argument to the second order and integrating over $\alpha$ we obtain $I \propto e^{-NL_w(\mu)}$ so that the survival probability behaves as

$$p_s(t) \sim e^{-\left(\lambda - \frac{L_W(\lambda\tau)}{\tau}\right)t} .$$

Using the expansion $L_W(x) = x - x^2 + O(x^3)$, we find that when $\lambda\tau \ll 1$ the survival probability behaves as

$$p_s(t) \sim e^{-\lambda^2 \tau t} .$$

## 1.3 Distribution of transit times

We now suppose that the cars or particles have a distribution of transit times, $\psi(\tau)$, where $\int_0^\infty \psi(\tau) d\tau = 1$ and for simplicity we assume that the creation rate $\lambda$ does not depend on $\tau$. The last of Eqs. (2) becomes

$$\frac{dq_s(n,t)}{dt} = \lambda \int_0^\infty \psi(\tau) q_s(n-1, t-\tau) e^{-\lambda\tau} d\tau - \lambda q_s(n,t), \;\; n \geq 2$$

with the other two unchanged. Taking the Laplace transform we obtain

$$\tilde{q_s}(n,u) = \left[\frac{\lambda}{\lambda+u} \int_0^\infty e^{-(\lambda+u)\tau} \psi(\tau) d\tau\right] \hat{q_s}(n-1,u) ,$$

which implies

$$\tilde{q_s}(n,u) = \frac{\lambda^n}{(\lambda+u)^{n+1}} \left[\int_0^\infty e^{-(\lambda+u)\tau} \psi(\tau) d\tau\right]^{n-1} , \;\; n \geq 1 ,$$

from which the mean survival time is found to be

$$\langle t \rangle = \tilde{G}(1,0) = \sum_{n=0}^\infty \tilde{q}_s(n,0) = \frac{2 - \tilde{\psi}(\lambda)}{\lambda(1 - \tilde{\psi}(\lambda))} .$$

To generalize Eq. (6) to a distribution of transit times, let $h(m, \tau_1, \tau_2, ..., \tau_{m+1})$ denote the probability that $m$ particles pass before failure and the transit times of the first $m+1$ particles are $\tau_1, \tau_2, ..., \tau_{m+1}$. Following the arguments given in the Letter

$$h(m, \tau_1, \tau_2, ..., \tau_{m+1}) = e^{-\lambda\tau_1} e^{-\lambda\tau_2} ... e^{-\lambda\tau_m} (1 - e^{-\lambda\tau_{m+1}}) .$$

Averaging over the transit times

$$\bar{h}(m) = \prod_{i=1}^{m+1} \int_0^\infty d\tau_i \; h(m, \tau_1, \tau_2, ..., \tau_{m+1}) = [\tilde{\psi}(\lambda)]^m (1 - \tilde{\psi}(\lambda)) \, .$$

from which we obtain Eq.(10).

# 2 Counterflow model

Let $p_k(n_1, n_2; t)$ denote the probability that the system has survived until time $t$ and $n_1$ particles of type 1 and $n_2$ of type 2 have entered the passage and the last particle to enter the passage was of type $k = 1, 2$. This choice provides a complete partition of the event space into disjoint events. Indeed at any time $t$, $(n_1, n_2) \cap$ (no traffic jam up to this time) for $n_1, n_2 \geq 0$ is a complete and disjoint partition of the event (no traffic jam up to this time). Moreover each event $(n_1, n_2)$ can be decomposed into the sum of the two disjoint subevents $(n_1, n_2, 1)$ and $(n_1, n_2, 2)$, indicating that at the given time $n_1$ and $n_2$ particles of respective type 1 and 2 entered the bridge, with the last one of type being respectively of type 1 and 2. Therefore we can write

$$p(n_1, n_2; t) = p_1(n_1, n_2; t) + p_2(n_1, n_2; t) \text{ for } n_1, n_2 \neq 0$$

$p(0, 0; t) = p_1(0, 0; t) = p_2(0, 0; t)$ (by convention) and

$$p_s(t) = \sum_{n_1=0}^{\infty} \sum_{n_2=0}^{\infty} p(n_1, n_2; t)$$

## 2.1 Generating function and survival probability

In order to solve the differential equations for $p_1(n_1, n_2; t)$ and $p_2(n_1, n_2; t)$, let us introduce the generating function

$$G(z_1, z_2; t) = \sum_{n_1=0}^{\infty} \sum_{n_2=0}^{\infty} z_1^{n_1} z_2^{n_2} p(n_1, n_2; t) \, .$$

It is convenient to decompose $G(z_1, z_2, t)$ in the following way:

$$G(z_1, z_2; t) = p(0, 0; t) + H_1(z_1; t) + H_2(z_2; t) + F_1(z_1, z_2; t) + F_2(z_1, z_2; t) \, , \tag{S2}$$

where

$$H_1(z_1; t) = \sum_{n_1=1}^{\infty} z_1^{n_1} p_1(n_1, 0; t)$$

$$H_2(z_2; t) = \sum_{n_2=1}^{\infty} z_2^{n_2} p_1(0, n_2; t)$$

$$F_k(z_1, z_2; t) = \sum_{n_1=1}^{\infty} \sum_{n_2=1}^{\infty} z_1^{n_1} z_2^{n_2} p_k(n_1, n_2; t) \text{ for } k = 1, 2$$

The Laplace transform in $t$ of Eq. (S2) is

$$\tilde{G}(z_1, z_2; u) = \tilde{p}(0, 0; u) + \tilde{H}_1(z_1; u) + \tilde{H}_2(z_2; u) + \tilde{F}_1(z_1, z_2; u) + \tilde{F}_2(z_1, z_2; u) \, , \tag{S3}$$

where

$$\tilde{p}(0,0;u) = \frac{1}{\lambda_1 + \lambda_2 + u}\,.$$

By using Eqs. (13) and the definition of $H_1(z;t)$, one obtains

$$\frac{dH_1(z;t)}{dt} = -[\lambda_1(1-z) + \lambda_2]H_1(z;t) + z\lambda_1 e^{-(\lambda_1+\lambda_2)t}$$

whose Laplace transform is given by

$$\tilde{H}_1(z;u)[u + \lambda_1(1-z) + \lambda_2] = \frac{z\lambda_1}{(\lambda_1+\lambda_2)+u}\,.$$

Inversion gives

$$H_1(z;t) = e^{-[\lambda_1(1-z)+\lambda_2]t} - e^{-(\lambda_1+\lambda_2)t}\,.$$

The probability $p_1(n_1, 0; t)$ can be obtained by using the following formula

$$p_1(n_1,0;t) = \frac{1}{n_1!}\left.\frac{dH(z,1;t)}{dz_1^n}\right|_{z=0}\,,$$

which gives

$$p_1(n_1,0;t) = {\lambda_1}^{n_1}\frac{t^{n_1}}{(n_1)!}e^{-(\lambda_1+\lambda_2)t}$$

Similarly, one finds that

$$H_2(z;t) = e^{-(\lambda_1+\lambda_2(1-z))t} - e^{-(\lambda_1+\lambda_2)t}$$

and

$$p_2(0,n_2;t) = {\lambda_2}^{n_2}\frac{t^{n_2}}{(n_2)!}e^{-(\lambda_1+\lambda_2)t}\,.$$

Given these solutions of the "boundary" equations, the "bulk" solutions can now be obtained.

By using Eqs. (12) and the corresponding differential equation for $p_2(n_1, n_2; t)$, one obtains the differential equations satisfied by $F_k(z_1, z_2; t)$:

$$\begin{aligned}\frac{dF_1(z_1,z_2;t)}{dt} &= -[\lambda_1(1-z_1)+\lambda_2]F_1(z_1,z_2;t)+\\ &+ \lambda_1 z_1 e^{-(\lambda_1+\lambda_2)\tau_2}[F_2(z_1,z_2;t-\tau_2) + H_2(z_2,t-\tau_2)]\\ \frac{dF_2(z_1,z_2;t)}{dt} &= -[\lambda_1+\lambda_2(1-z_2)]F_2(z_1,z_2;t)+\\ &+ \lambda_2 z_2 e^{-(\lambda_1+\lambda_2)\tau_1}[F_1(z_1,z_2;t-\tau_1) + H_1(z_1,t-\tau_1)]\,.\end{aligned}$$

The Laplace transform of these equations can be written in matrix form: $\mathsf{A}\tilde{\mathbf{F}} = \tilde{\mathbf{B}}$ where

$$\tilde{\mathbf{F}} = \begin{pmatrix} \tilde{F}_1(z_1,z_2;u) \\ \tilde{F}_2(z_1,z_2;u) \end{pmatrix}$$

and

$$\tilde{\mathbf{B}} = \begin{pmatrix} \lambda_1 z_1 e^{-(\lambda_1+\lambda_2+u)\tau_2}\tilde{H}_2(z_2;u) \\ \lambda_2 z_2 e^{-(\lambda_1+\lambda_2+u)\tau_1}\tilde{H}_1(z_1;u) \end{pmatrix}$$

are two-dimensional vectors, and the matrix $\mathsf{A}$ is given by

$$\mathsf{A} = \begin{pmatrix} u+\lambda_1(1-z_1)+\lambda_2 & -\lambda_1 z_1 e^{-(\lambda_1+\lambda_2+u)\tau_2} \\ -\lambda_2 z_2 e^{-(\lambda_1+\lambda_2+u)\tau_1} & u+\lambda_1+\lambda_2(1-z_2)\,. \end{pmatrix}$$

The solution of the linear system is

$$\tilde{F}_1(z_1,z_2,u) = \frac{\lambda_1\lambda_2 z_1 z_2}{\Delta(\lambda_1+\lambda_2+u)}\left[e^{-(\lambda_1+\lambda_2+u)\tau_2} + \frac{\lambda_1 z_1 e^{-(\lambda_1+\lambda_2+u)(\tau_1+\tau_2)}}{u+\lambda_2+\lambda_1(1-z_1)}\right]$$
$$\tilde{F}_2(z_1,z_2,u) = \frac{\lambda_1\lambda_2 z_1 z_2}{\Delta(\lambda_1+\lambda_2+u)}\left[e^{-(\lambda_1+\lambda_2+u)\tau_1} + \frac{\lambda_1 z_1 e^{-(\lambda_1+\lambda_2+u)(\tau_1+\tau_2)}}{u+\lambda_1+\lambda_2(1-z_2)}\right]$$

where

$$\Delta = (u+\lambda_2+\lambda_1(1-z_1))(u+\lambda_1+\lambda_2(1-z_2)) - \lambda_1\lambda_2 z_1 z_2 e^{-(\lambda_1+\lambda_2+u)(\tau_1+\tau_2)}\,.$$

Introducing these results into Eq. (S3), we obtain the generating function, Eq. (15).

From $p_s(t) = G(1,1,t)$ we find the survival probability

$$\tilde{p}_s(u) = \frac{1}{\lambda_1+\lambda_2+u}\left(1 + \sum_{k=0}^{\infty}\frac{(\lambda_1\lambda_2)^k e^{-k(\lambda_1+\lambda_2+u)(\tau_1+\tau_2)}}{[(u+\lambda_2)(u+\lambda_1)]^k}\left(\frac{\lambda_2}{u+\lambda_1}+\frac{\lambda_1}{u+\lambda_2}\right)\right.$$
$$\left. + \sum_{k=0}^{\infty}\frac{(\lambda_1\lambda_2)^{k+1} e^{-k(\lambda_1+\lambda_2+u)(\tau_1+\tau_2)}}{[(u+\lambda_2)(u+\lambda_1)]^{k+1}}\left(e^{-(\lambda_1+\lambda_2+u)\tau_2} + e^{-(\lambda_1+\lambda_2+u)\tau_1}\right)\right)\,, \quad \text{(S4)}$$

where we have used

$$\frac{\lambda_1\lambda_2}{(u+\lambda_1)(u+\lambda_2) - \lambda_1\lambda_2 e^{-(\lambda_1+\lambda_2+u)(\tau_1+\tau_2)}} = \sum_{k=0}^{\infty}\frac{(\lambda_1\lambda_2)^{k+1} e^{-k(\lambda_1+\lambda_2+u)(\tau_1+\tau_2)}}{[(u+\lambda_2)(u+\lambda_1)]^{k+1}}\,.$$

This form allows the inversion of the Laplace transform in the following two cases:

a) ($\lambda_1 = \lambda_2 = \lambda$) The Laplace transform of the survival probability may be inverted by using partial fraction decomposition:

$$\frac{\lambda_1^n}{(u+\lambda)^n(u+2\lambda)} = \frac{(-1)^n}{(u+2\lambda)} + \sum_{k=1}^{n}\frac{(-1)^{n-1}\lambda^{k-1}}{(u+\lambda)^k}\,.$$

The inverse Laplace transform of the rhs is then given by

$$(-1)^n e^{-2\lambda t} + e^{-\lambda t}\sum_{k=1}^{n}\frac{(-1)^{n-k}}{(k-1)!}(\lambda t)^{k-1}$$

Using this in Eq. (S4) gives

$$p_s(t) = e^{-2\lambda t} + \sum_{k=0}\theta(t-k(\tau_1+\tau_2))\left(-2e^{-2\lambda t} + 2e^{-\lambda(t+k(\tau_1+\tau_2))}\sum_{l=0}^{2k}\frac{(-1)^l}{l!}(\lambda(t-k(\tau_1+\tau_2)))^l\right)$$
$$+ \sum_{k=0}\theta(t-(k+1)\tau_1-k\tau_2)\left(e^{-2\lambda t} - e^{-\lambda(t+(k+1)\tau_1+k\tau_2)}\sum_{l=0}^{2k+1}\frac{(-1)^l}{l!}(\lambda(t-(k+1)\tau_1-k\tau_2))^l\right)$$
$$+ \sum_{k=0}\theta(t-k\tau_1-(k+1)\tau_2)\left(e^{-2\lambda t} - e^{-\lambda(t+k\tau_1+(k+1)\tau_2)}\sum_{l=0}^{2k+1}\frac{(-1)^l}{l!}(\lambda(t-k\tau_1-(k+1)\tau_2))^l\right)\,.$$

b) $\lambda_1 \neq \lambda_2$. To obtain the result in this case we need to perform the partial fraction decomposition of

$$\frac{\lambda_1^p\lambda_2^n}{(u+\lambda_1)^n(u+\lambda_2)^p(u+\lambda_1+\lambda_2)} = \frac{d}{(u+\lambda_1+\lambda_2)} + \sum_{k=1}^{n}\frac{\lambda_2^{k-1}\mu_k}{(u+\lambda_1)^k} + \sum_{k=1}^{p}\frac{\lambda_1^{k-1}\nu_k}{(u+\lambda_2)^k} \quad \text{(S5)}$$

where $p = n, n \pm 1$. We obtain that $d = (-1)^{p+n}$,

$$\mu_k = (-1)^{n-k}\left(\frac{\lambda_1}{\lambda_2}\right)^p \sum_{r=0}^{n-k}\left(1-\frac{\lambda_1}{\lambda_2}\right)^{-(r+p)}\frac{(p-1+r)!}{r!(p-1)!}$$

and

$$\nu_k = (-1)^{p-k}\left(\frac{\lambda_2}{\lambda_1}\right)^n \sum_{s=0}^{p-k}(1-\frac{\lambda_2}{\lambda_1})^{-(s+n)}\frac{(n-1+s)!}{s!(n-1)!}$$

The inverse Laplace transform of the rhs of Eq. (S5) is then given by

$$(-1)^{n-p}e^{-(\lambda_1+\lambda_2)t} + e^{-\lambda_1 t}\sum_{k=0}^{n-1}\frac{\mu_{k+1}(\lambda_2 t)^k}{k!} + e^{-\lambda_2 t}\sum_{k=0}^{p-1}\frac{\nu_{k+1}(\lambda_1 t)^k}{k!}$$

Note that the above equation vanishes when $t$ goes to 0. Applying these results in Eq. (S4) we obtain

$$\begin{aligned}
p_s(t) = e^{-(\lambda_1+\lambda_2)t} + \Bigg(&\sum_{k=0}\theta(t-k(\tau_1+\tau_2))a_k(t-k(\tau_1+\tau_2))e^{-k(\lambda_1+\lambda_2)(\tau_1+\tau_2)} \\
&+\sum_{k=0}\theta(t-(k+1)\tau_1-k\tau_2)b_{k+1}(t-(k+1)\tau_1-k\tau_2)e^{-(k+1)\lambda_1\tau 1-k\lambda_2\tau_2} \\
&+\sum_{k=0}\theta(t-k\tau_1-(k+1)\tau_2)b_{k+1}(t-k\tau_1-(k+1)\tau_2)e^{-k\lambda_1\tau 1-(k+1)\lambda_2\tau_2}\Bigg)
\end{aligned}$$

where

$$\begin{aligned}
a_k(t) =& -2e^{-(\lambda_1+\lambda_2)t} + e^{-\lambda_1 t}\Bigg[\sum_{l=0}^{k-1}\frac{(\lambda_2 t)^l}{l!}\left(\frac{\lambda_1}{\lambda_2}\right)^{k+1}(-1)^{k-l-1}\sum_{r=0}^{k-1-l}\left(1-\frac{\lambda_1}{\lambda_2}\right)^{-(r+k+1)}\frac{(k+r)!}{r!k!} \\
&+\sum_{l=0}^{k}\frac{(\lambda_2 t)^l}{l!}\left(\frac{\lambda_1}{\lambda_2}\right)^{k}(-1)^{k-l}\sum_{r=0}^{k-l}\left(1-\frac{\lambda_1}{\lambda_2}\right)^{-(r+k)}\frac{(k-1+r)!}{r!(k-1)!}\Bigg] \\
&+e^{-\lambda_2 t}\Bigg[\sum_{m=0}^{k}\frac{(\lambda_1 t)^m}{m!}(-1)^{k-m}\left(\frac{\lambda_2}{\lambda_1}\right)^{k}\sum_{s=0}^{k-m}(1-\frac{\lambda_2}{\lambda_1})^{-(s+k)}\frac{(k-1+s)!}{s!(k-1)!} \\
&+\sum_{m=0}^{k-1}\frac{(\lambda_1 t)^m}{m!}(-1)^{k+1-m}\left(\frac{\lambda_2}{\lambda_1}\right)^{k+1}\sum_{s=0}^{k-1-m}(1-\frac{\lambda_2}{\lambda_1})^{-(s+k+1)}\frac{(k+s)!}{s!k!}\Bigg]
\end{aligned}$$

and

$$\begin{aligned}
b_k(t) =& e^{-(\lambda_1+\lambda_2)t} - e^{-\lambda_1 t}\sum_{l=0}^{k-1}\frac{(\lambda_2 t)^l}{l!}(-1)^{k-l-1}\left(\frac{\lambda_1}{\lambda_2}\right)^{k+1}\sum_{r=0}^{k-1-l}\left(1-\frac{\lambda_1}{\lambda_2}\right)^{-(r+k+1)}\frac{(k+r)!}{r!k!} \\
&- e^{-\lambda_2 t}\sum_{m=0}^{k-1}\frac{(\lambda_1 t)^m}{m!}(-1)^{k-m-1}\left(\frac{\lambda_2}{\lambda_1}\right)^{k+1}\sum_{s=0}^{k-m-1}(1-\frac{\lambda_2}{\lambda_1})^{-(s+k+1)}\frac{(k+s)!}{s!k!}\,.
\end{aligned}$$

## 2.2 Calculation of $h(m_1, m_2)$

To calculate e.g. $h(1,0)$ we must take into account two types of event sequences: see Fig. 1. Type one consists of the entry of $n \geq 2$ particles of type 1 on the left followed by a particle of type 2 on the right.

It is the entry of the last particle that leads to failure. For example let us consider $n = 2$ and let $t_1$ and $t_2$ denote the times between the events. Then to achieve the desired sequence we must have $t_1 + t_2 > \tau_1$ to allow the first particle to pass and $t_2 < \tau_1$ to cause failure. Given that the event density at time $t$ is $(\lambda_1 + \lambda_2)e^{-(\lambda_1+\lambda_2)t}$, the probability of the sequence is

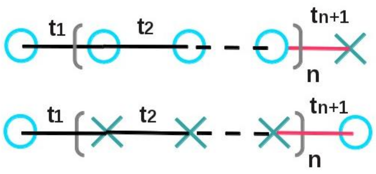


Figure 1: Event sequences that contribute to $h(1, 0)$. Circles represent the entry of a species of type 1 on the left and crosses corresond to species of type 2 entering on the right hand side.

$$(\lambda_1 + \lambda_2)^2 \int_0^\infty dt_1 \int_0^\infty dt_2\, p_1 e^{-(\lambda_1+\lambda_2)t_1} p_1 e^{-(\lambda_1+\lambda_2)t_2} p_2 \theta(t_1 + t_2 - \tau_1)\theta(\tau_1 - t_2) \\ = p_1^2 p_2 (\lambda_1 + \lambda_2)\tau_1 e^{-(\lambda_1+\lambda_2)\tau_1} \,,$$

where $p_k = \lambda_k/(\lambda_1 + \lambda_2)$ and $\theta(x)$ is the heaviside function.

Generalizing to $n$ and summing gives

$$\pi_1^{(1,0)} = \sum_{n=1}^{\infty} p_1 p_2 \frac{[(\lambda_1 + \lambda_2)\tau_1]^n}{n!} p_1^n e^{-(\lambda_1+\lambda_2)\tau_1} \\ = p_1 p_2 e^{-(\lambda_1+\lambda_2)\tau_1} [e^{\lambda_1\tau_1} - 1] \,.$$

The second possibility is for a particle of type 1 to enter on the left, followed by one or more particles of type 2 on the right and finally another particle of type 1 to cause failure. In this case we obtain:

$$\pi_2^{(1,0)} = \sum_{n=1}^{\infty} p_1 p_2^n p_1 e^{-(\lambda_1+\lambda_2)\tau_1} (1 - \alpha_n e^{-(\lambda_1+\lambda_2)\tau_2}) \\ = p_1 p_2 e^{-(\lambda_1+\lambda_2)\tau_1} (1 - e^{-\lambda_1\tau_2}) \,,$$

where

$$\alpha_n = \sum_{k=1}^{n} \frac{(\lambda_1 + \lambda_2)^{k-1}}{(k-1)!} \,.$$

Finally

$$h(1, 0) = \pi_1^{(1,0)} + \pi_2^{(1,0)} = p_1 p_2 (e^{-\lambda_2\tau_1} - e^{-(\lambda_1+\lambda_2)\tau_1} e^{-\lambda_1\tau_2})$$

and $h(0, 1)$ can be written down directly by symmetry. The results can then be generalized to $h(n_1, 0)$ and $h(0, n_2)$ by noting that the additional particles (type 1 and 2, respectively) must be introduced at the beginning of the sequence. The same approach can be used to obtain $h(1, 1)$ but it is tedious to go further.
